# Supplementary material for: MS-COOT: Comparing Morse-Smale Complexes with Co-Optimal Transport
Source: arXiv:2606.08258 source file (2026-10-24)
Supplement: Supplementary file 1 [file supplementary.tex]

\documentclass[journal,review]{vgtc}     
\onlineid{1476}
\vgtccategory{Research}
\usepackage{amsmath, amssymb}
\usepackage{amsfonts}
\usepackage{tikz}
\usepackage{multirow}
\usetikzlibrary{arrows.meta, positioning, calc}
\usepackage{booktabs}
\usepackage{graphicx}

\newcommand{\para}[1]{\vspace{1mm}\noindent{\textbf{#1}}}

\graphicspath{{figs/}{figures/}{./}}

\begin{document}
\title{Supplementary Material for\\MS-COOT: Comparing Morse-Smale Complexes with Co-Optimal Transport}
\author{Anonymous Submission}
\maketitle

This document provides supplementary material,
including notation (\cref{sec:notation}),
implementation details (\cref{sec:appendix_implementation}),
and additional TOSCA results (\cref{sec:appendix_tosca}).

\section{Notation}
\label{sec:notation}
\Cref{tab:notation} summarizes the notation used throughout the main paper.

\begin{table}[hbt]
\centering
\caption{Summary of notation.}
\label{tab:notation}
\small
\setlength{\tabcolsep}{4pt}
\renewcommand{\arraystretch}{1}
\begin{tabular}{@{}lp{5.2cm}@{}}
\toprule
\textbf{Symbol} & \textbf{Description} \\
\midrule
\multicolumn{2}{l}{\textit{Input and Morse-Smale Complex}} \\
$f, g$ & Scalar fields \\
$\mathrm{CP}_i$ & The $i$-th critical point \\
$R_j$ & The $j$-th region (2-cell in 2D, 3-cell in 3D) \\
$\partial R_j$ & Set of boundary CPs of region $R_j$ \\
$n, m$ & Number of CPs and regions \\
$n_f, n_g, m_f, m_g$ & Number of CPs and regions for $f$ and $g$ \\
$\mathrm{type}(\cdot)$ & CP type: 0\,(min), 1\,(saddle), 2\,(max) in 2D; 0/1/2/3 in 3D \\
$\mathrm{pers}(\cdot)$ & Persistence: $|f(\text{birth}) - f(\text{death})|$ \\
\midrule
\multicolumn{2}{l}{\textit{Hypernetwork and Augmented Graph}} \\
$\mathcal{H}_f, \mathcal{H}_g$ & Measure hypernetworks $(V, E, \mu, \nu, \omega)$ \\
$V,\; E$ & Node set (CPs) and hyperedge set (regions) \\
$G = (V_G, E_G)$ & Augmented graph; $V_G = V \cup \{\mathrm{VC}_j\}$ \\
$\mathrm{VC}_j$ & Virtual region center of $R_j$ \\
$d_G(\cdot,\cdot)$ & Shortest-path distance on $G$ \\
$\omega \in \mathbb{R}^{n \times m}$ & Hypernetwork function; $\omega[i,j] = d_G(\mathrm{CP}_i, \mathrm{VC}_j)$ \\
$Z$ & Joint normalization factor: $\max(\max_{i,k} \omega_f[i,k],$ $\max_{j,l} \omega_g[j,l])$ \\
\midrule
\multicolumn{2}{l}{\textit{Measures}} \\
$\mu \in \mathbb{R}^{n}$ & Node measure on CPs (persistence-based) \\
$\nu \in \mathbb{R}^{m}$ & Hyperedge measure on regions (from $\mu$) \\
$\sigma$ & PI Gaussian kernel bandwidth \\
\midrule
\multicolumn{2}{l}{\textit{MS-COOT Formulation}} \\
$\pi \in \mathbb{R}^{n_f \times n_g}$ & CP coupling \\
$\xi \in \mathbb{R}^{m_f \times m_g}$ & Region coupling \\
$\Pi(\mu_f, \mu_g)$ & Set of couplings with marginals $\mu_f, \mu_g$ \\
$C \in \mathbb{R}^{n_f \times n_g}$ & Sample cost (type penalty or scalar difference) \\
$\alpha$ & Balance weight (structure vs.\ sample cost) \\

$\varepsilon$ & Sinkhorn regularization parameter \\
\bottomrule
\end{tabular}
\end{table}

\section{Implementation Details}
\label{sec:appendix_implementation}

This section provides implementation details for reproducing the experiments in the main paper. 
All experiments are performed on an Intel i9-12900K CPU with 128\,GB RAM.

\para{Parameter settings.}
\Cref{tab:params} summarizes the MS-COOT parameters, which are shared across all five datasets; the only dataset-specific parameter is the persistence simplification threshold (\cref{tab:persistence}). 

The Sinkhorn regularization $\varepsilon = 0.001$ follows standard practice in optimal transport~\cite{cuturi2013sinkhorn}, balancing numerical stability and approximation quality. 
If Sinkhorn diverges, we fall back to exact EMD ($\varepsilon = 0$). 
The balance weight $\alpha = 0.5$ assigns equal importance to structural consistency and node-level constraints. 
The PI bandwidth $\sigma = 0.3$ emphasizes high-persistence critical points while retaining contributions from lower-persistence features. 
The persistence image is computed on a $100{\times}100$ grid with scalar values normalized to $[0,1]$~\cite{adams2017persistence}.

The remaining solver parameters (50 BCD iterations, 200 Sinkhorn iterations, and $10^{-7}$ convergence tolerance) serve as upper bounds; in practice, convergence is typically reached earlier. 
Parameter sensitivity is evaluated on TOSCA (Figure~10 in the main paper), where $\alpha$, $\sigma$, and $\varepsilon$ exhibit stable performance across a broad range: accuracy remains above 80\% for $\alpha \in [0.3,0.9]$, $\sigma \in [0.2,0.6]$, and $\varepsilon \in \{0, 0.001, 0.01\}$. 
Because these parameters are robust on TOSCA, which is the dataset with the most diverse MS structures, we use the same defaults for all other datasets without further tuning. 
This transferability is supported by the Viscous Finger experiment, where the same parameters yield 80\% classification accuracy on an independent 3D volumetric dataset (Table~2 in the main paper).

\begin{table}[hbt]
\centering
\caption{Parameter settings for MS-COOT (shared across all datasets).}
\label{tab:params}
\small
\begin{tabular}{@{}lr@{}}
\toprule
\textbf{Parameter} & \textbf{Value} \\
\midrule
Sinkhorn regularization ($\varepsilon$) & 0.001 \\
Sample cost weight ($\alpha$) & 0.5 \\
PI bandwidth ($\sigma$) & 0.3 \\
PI grid resolution & $100 \times 100$ \\
Max BCD iterations & 50 \\
Max Sinkhorn iterations & 200 \\
Convergence tolerance & $10^{-7}$ \\
\bottomrule
\end{tabular}
\end{table}

\para{Persistence simplification.}
\Cref{tab:persistence} reports the persistence thresholds for each dataset, expressed as a percentage of the global scalar range, along with the average number of critical points and regions before and after simplification. 
Persistence simplification~\cite{edelsbrunner2002topological} removes low-persistence features by canceling saddle-extremum pairs, yielding a coarser MS complex that preserves prominent structures.

Thresholds are selected by inspecting persistence curves (number of surviving features versus threshold) and choosing the elbow point where the decay transitions from rapid to gradual, following~\cite{lukasczyk2020localized}. 
Lower thresholds (1\%) suffice for Vortex Street and TOSCA due to relatively clean scalar fields, while higher thresholds (6-7\%) are required for simulation datasets to suppress numerical noise. 
A systematic study of threshold sensitivity is left for future work; the TOSCA ablation (Figure~10) indicates that MS-COOT is robust to moderate parameter variation.

\begin{table}[hbt]
\centering
\caption{Persistence simplification thresholds and their effect on MS complex size. Threshold is a percentage of the global scalar range. Avg CPs and Avg Regions report the mean count per instance before and after simplification.}
\label{tab:persistence}
\small
\setlength{\tabcolsep}{3pt}
\begin{tabular}{@{}lc rr rr@{}}
\toprule
 & & \multicolumn{2}{c}{Before simpl.} & \multicolumn{2}{c}{After simpl.} \\
\cmidrule(lr){3-4} \cmidrule(lr){5-6}
Dataset & Thresh. & CPs & Reg. & CPs & Reg. \\
\midrule
Vortex Street    & 1\%    & 142 & 102 & 117 & 89  \\
Ionization Front & 7\%    & 516 & 270 & 34  & 29  \\
Heated Cylinder  & 6.5\%  & 282 & 164 & 45  & 31  \\
TOSCA            & 1\%    & 93  & 62  & 43  & 37  \\
Viscous Finger   & 6\%    & 656 & 105 & 466 & 10  \\
\bottomrule
\end{tabular}
\end{table}

\begin{table}[hbt]
\centering
\caption{Dataset statistics and per-pair runtime (mean $\pm$ std over 5 runs, in ms).
$N$: number of instances.
Reg.: regions.
VS: Vortex Street, IF: Ionization Front, HC: Heated Cylinder, VF: Viscous Finger.
All instances are timesteps except TOSCA (meshes).}
\label{tab:implementation}
\footnotesize
\setlength{\tabcolsep}{2.5pt}
\renewcommand{\arraystretch}{0.95}
\begin{tabular}{lccc cccc}
\toprule
 & & Avg & Avg & \multicolumn{4}{c}{Runtime (ms/pair)} \\
\cmidrule(lr){5-8}
Dataset & $N$ & CPs & Reg. & WD & GWD & FGW & MS-COOT \\
\midrule
VS    & 157 & 117 & 89  & $0.9{\pm}0.6$   & $16{\pm}17$     & $6.5{\pm}2.6$   & $62{\pm}17$ \\
IF    & 30  & 34  & 29  & $0.6{\pm}0.2$   & $1.4{\pm}0.9$   & $0.6{\pm}0.5$   & $25{\pm}6$ \\
HC    & 100 & 45  & 31  & $0.4{\pm}0.1$   & $1.2{\pm}0.9$   & $0.8{\pm}0.5$   & $43{\pm}1$ \\
TOSCA & 80  & 43  & 37  & $0.2{\pm}0.1$   & $1.6{\pm}1.1$   & $0.8{\pm}0.6$   & $34{\pm}0.2$ \\
VF    & 120 & 466 & 10  & $13{\pm}7$      & $1119{\pm}604$  & $230{\pm}105$   & $1058{\pm}73$ \\
\bottomrule
\end{tabular}
\end{table}

\para{Baselines and runtime.}
All baselines use uniform node weights ($\mu_i = 1/n$). 
For WD, the cost matrix is the $\ell_2$ distance between CP coordinates, normalized by the diagonal of the bounding box (402.0 for Vortex Street, 649.3 for Ionization Front, 3.162 for Heated Cylinder, and per-mesh for TOSCA and Viscous Finger). 

For GWD, intra-space distances are defined as shortest-path distances on the Euclidean-weighted 1-skeleton, normalized to $[0,1]$ by dividing by the maximum value. 
For disconnected components, infinite distances are replaced by twice the maximum finite distance. 
For FGW, the feature and structure costs follow WD and GWD, respectively, with the trade-off parameter set to 0.5. 
All baseline solvers use exact EMD (no entropic regularization).

\Cref{tab:implementation} reports dataset statistics and per-pair runtimes. 
MS-COOT is approximately 5–50$\times$ slower than FGW, due to the additional region coupling and BCD iterations. 
On the largest dataset (Viscous Finger, average 466 CPs), MS-COOT requires approximately one second per pair, remaining practical for moderate-scale ensemble analysis.

\begin{figure}[t!]
  \centering
  \includegraphics[width=0.85\columnwidth]{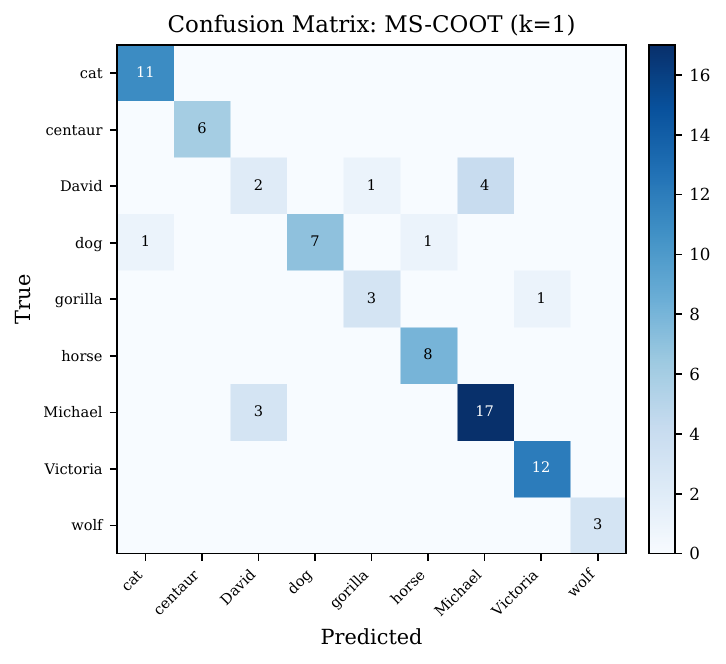}
    \caption{\textbf{MS-COOT confusion matrix on TOSCA} ($k{=}1$, leave-one-out). Five categories achieve perfect recall. The main confusion is David\,$\to$\,Michael (4 of 7), reflecting their nearly identical MS topology.}
  \label{fig:tosca_confusion}
\end{figure}

\begin{figure}[hbt!]
  \centering
  \includegraphics[width=\columnwidth]{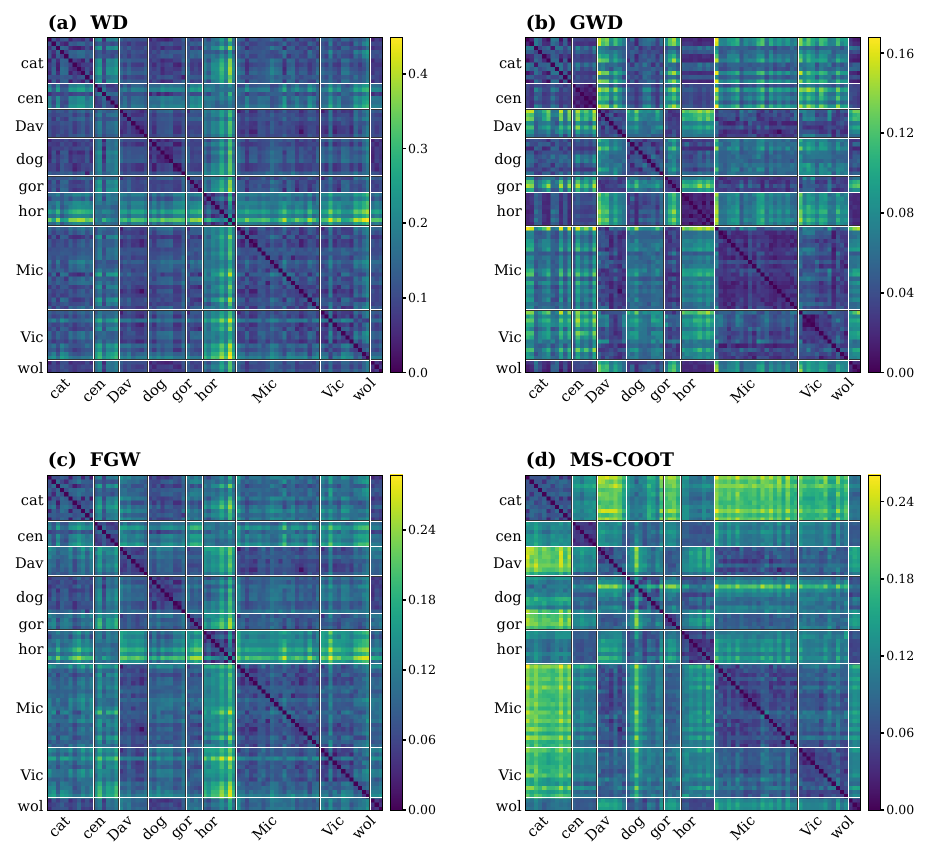}
  \caption{\textbf{Pairwise distance matrices on TOSCA} for (a)~WD, (b)~GWD, (c)~FGW, and (d)~MS-COOT. 
Rows and columns are ordered by category: cat~(11), centaur~(6), David~(7), dog~(9), gorilla~(4), horse~(8), Michael~(20), Victoria~(12), and wolf~(3); white lines separate category blocks. 
Dark diagonal blocks indicate low within-class distances. 
MS-COOT shows clear separation between categories with fewer low-distance off-diagonal regions, consistent with its higher classification accuracy (Table~1 in the main paper). 
The relatively low distance between the David and Michael blocks across all methods reflects their similar MS topology.}
  \label{fig:tosca_distmat}
\end{figure}

\begin{figure}[hbt!]
  \centering
  \includegraphics[width=\columnwidth]{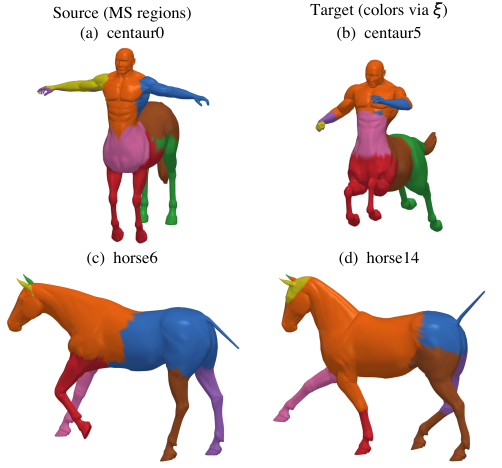}
  \caption{\textbf{MS-COOT intra-class region correspondence on TOSCA.} 
  Left: source shapes colored by MS regions. Right: target shapes colored via transfer through the region coupling~$\xi$.
(a,b)~Centaur shapes: MS-COOT preserves the relative spatial arrangement of regions (e.g., upper body vs.\ lower body), resulting in consistent correspondence of major parts despite pose variation. 
(c,d)~Horse shapes: limb and body regions are consistently aligned across poses, with colors preserved along corresponding legs and torso regions; minor differences reflect variations in the underlying segmentation.}
  \label{fig:tosca_intra}
\end{figure}

\begin{figure}[hbt!]
  \centering
  \includegraphics[width=\columnwidth]{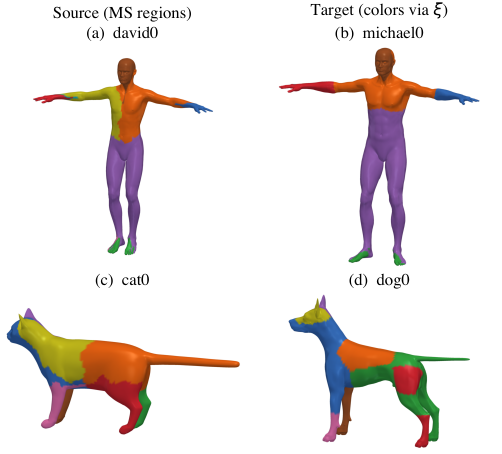}
  \caption{
  \textbf{MS-COOT inter-class region correspondence on TOSCA.}
  Left: source shapes colored by MS regions. Right: target shapes colored via transfer through the region coupling~$\xi$.
  (a,b)~David $\rightarrow$ Michael: regions align at a coarse level (upper vs.\ lower body), with consistent mapping of legs and partial alignment of arms. 
  (c,d)~Cat $\rightarrow$ Dog: correspondences capture partial similarity in head and limb regions, while other regions exhibit less consistent alignment due to morphological differences.}
  \label{fig:tosca_inter}
\end{figure}

\section{TOSCA: Additional Results}
\label{sec:appendix_tosca}

\para{Confusion matrix.}
\Cref{fig:tosca_confusion} shows the full confusion matrix for MS-COOT on TOSCA with $k{=}1$ leave-one-out classification.
Five of nine categories achieve perfect recall (cat, centaur, horse, Victoria, wolf).
The primary source of error is David\,$\to$\,Michael: 4 of 7 David meshes are misclassified as Michael.
Both are male humanoid shapes with similar limb structure, resulting in nearly identical MS complexes under the AGD scalar field.
This confusion reflects a fundamental similarity in the topological structure of these shapes rather than a limitation specific to MS-COOT.

\para{Pairwise distance matrix.}
\Cref{fig:tosca_distmat} shows pairwise distance matrices for all 80 TOSCA meshes under WD, GWD, FGW, and MS-COOT, with rows and columns ordered by category label. 
Dark diagonal blocks indicate that within-class distances are generally smaller than between-class distances across methods. 
The David-Michael block exhibits relatively low between-class distance in all four methods, consistent with the classification confusion discussed above. 

While all methods exhibit block-diagonal structure to various extent, their cross-class behavior differs. 
WD and FGW produce more diffuse patterns outside the diagonal blocks, indicating weaker separation between categories. 
GWD shows many low-distance off-diagonal blocks, reflecting higher similarity between different classes. 
In contrast, MS-COOT shows fewer such off-diagonal low-distance regions, indicating reduced cross-class similarity and aligning with its improved classification performance on this dataset.

\para{Region correspondence.}
\Cref{fig:tosca_intra,fig:tosca_inter} visualize the region coupling~$\xi$ for representative intra-class and inter-class TOSCA shape pairs. 
In each case, the source mesh is colored by MS regions, and the target mesh inherits these colors through $\xi$, illustrating the induced region correspondences.

For intra-class pairs (\cref{fig:tosca_intra}), MS-COOT preserves the relative spatial arrangement of regions across poses. 
Major structures, such as the upper and lower body in the centaur shapes and the torso and limbs in the horse shapes, are consistently aligned despite non-rigid deformation, with minor variations confined to small or boundary regions.

For inter-class pairs (\cref{fig:tosca_inter}), the correspondences reflect similarities at a coarser structural level. 
The David-Michael pair exhibits similar region organization, leading to consistent coarse alignment and explaining the observed classification confusion (\cref{fig:tosca_confusion}). 
In contrast, the cat-dog pair shows only partial correspondence: some regions (e.g., head and limbs) align, while others exhibit more ambiguous matches due to differences in morphology.

These examples illustrate that MS-COOT captures region-level relationships through spatial organization, producing meaningful correspondences within classes and interpretable partial alignment across different shape categories.

%% ============================================================
%%  REFERENCES (use same .bib as main paper)
%% ============================================================
\bibliographystyle{abbrv-doi-hyperref}
\bibliography{VIS'26-MSCOOT}
 
\end{document}
